# Supplementary material for: Ultrafast Hot Phonon Dynamics in MgB$_2$ Driven by Anisotropic Electron-Phonon Coupling
Source: arXiv:1904.03062 ancillary file (2020-01-30)
Supplement: Supplementary file 1 [file SuppInfo.pdf]

# Supplemental Material: Ultrafast Hot Phonon Dynamics in $MgB_2$ Driven by Anisotropic Electron-Phonon Coupling

D. Novko,[1,2,*] F. Caruso,[3] C. Draxl,[3] and E. Cappelluti[4,†]

[1] *Center of Excellence for Advanced Materials and Sensing Devices, Institute of Physics, Bijenička 46, 10000 Zagreb, Croatia*
[2] *Donostia International Physics Center (DIPC), Paseo Manuel de Lardizabal 4, 20018 Donostia-San Sebastián, Spain*
[3] *Institut für Physik and IRIS Adlershof, Humboldt-Universität zu Berlin, Berlin, Germany*
[4] *Istituto di Struttura della Materia, CNR, Division of Ultrafast Processes in Materials (FLASHit), 34149 Trieste, Italy*

## S1. FIRST-PRINCIPLES CALCULATION OF THE THERMODYNAMICS AND ELECTRON-PHONON PARAMETERS OF THE THEREE-TEMPERATURE MODEL

The specific heat capacities for the electron ($C_\mathrm{e}$) hot-phonon ($C_{E_{2g}}$) and cold-phonon ($C_\mathrm{ph}$) degrees of freedom are computed as [S1, S2]:

$$C_\mathrm{e} = \int_{-\infty}^{\infty} d\varepsilon N(\varepsilon)\varepsilon \frac{\partial f(\varepsilon-\mu;T_\mathrm{e})}{\partial T_\mathrm{e}}, \tag{S1}$$

$$C_{E_{2g}} = \int_0^{\infty} d\omega F_{E_{2g}}(\omega)\omega \frac{\partial b(\omega;T_{E_{2g}})}{\partial T_{E_{2g}}}, \tag{S2}$$

$$C_\mathrm{ph} = \int_0^{\infty} d\omega F_\mathrm{ph}(\omega)\omega \frac{\partial b(\omega;T_\mathrm{ph})}{\partial T_\mathrm{ph}}, \tag{S3}$$

where $N(\varepsilon)$ is the electronic density of states, $\mu$ the electronic chemical potential, and $f(x;T) = 1/[\exp(x/T)+1]$, $b(x;T) = 1/[\exp(x/T)-1]$ are the Fermi-Dirac and the Bose-Einstein distribution functions, respectively.

In similar way, one can compute the temperature-dependent electron-phonon relaxation rates as:

$$G_{E_{2g}} = \frac{2\pi k_B}{\hbar N(\mu)} \int d\Omega \Omega \alpha^2 F_{E_{2g}}(\Omega) \int_{-\infty}^{\infty} d\varepsilon N^2(\varepsilon) \frac{\partial f(\varepsilon-\mu;T_\mathrm{e})}{\partial T_\mathrm{e}}, \tag{S4}$$

$$G_\mathrm{ph} = \frac{2\pi k_B}{\hbar N(\mu)} \int d\Omega \Omega \alpha^2 F_\mathrm{ph}(\Omega) \int_{-\infty}^{\infty} d\varepsilon N^2(\varepsilon) \frac{\partial f(\varepsilon-\mu;T_\mathrm{e})}{\partial T_\mathrm{e}}. \tag{S5}$$

The detailed temperature dependence of all these quantities, obtained from the first-principles calculations, is shown in Fig. S1. The specific heat $C_\mathrm{e}$ scales in a good approximation linearly with $T_\mathrm{e}$ according the standard rule $C_\mathrm{e} = \gamma_\mathrm{e} T_\mathrm{e}$, where $\gamma_\mathrm{e} = 90\,\mathrm{J/m^3K^2}$. In the physical range we are interested in (300 K $\lesssim T_\mathrm{e} \lesssim$ 2000 K), the lattice specific heats

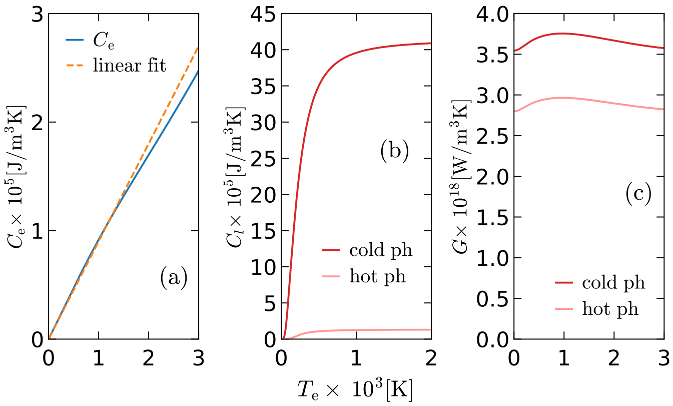


FIG. S1. (a) The specific heat capacity for the electrons $C_\mathrm{e}$ as a function of electron temperature $T_\mathrm{e}$ [Eq. (S1)]. The linear fit $C_\mathrm{e} = 90\,\mathrm{J/m^3K^2} \times T_\mathrm{e}$ is also shown. (b) The specific heat capacities for the hot- (light red) and cold-phonons (red) as a function of electron temperature $T_\mathrm{e}$ [Eqs. (S2) and (S3)]. (c) Temperature-dependent electron-phonon relaxation rates for the hot- and cold-phonon subsystems [Eqs. (S4) and (S5)].

$C_{E_{2g}}$, $C_{\rm ph}$, and the relaxation rates $G_{E_{2g}}$, $G_{\rm ph}$ are also almost temperature independent. We can thus reasonably evaluate the relaxation rates at zero temperature,

$$G_{E_{2g}} = \frac{2\pi k_B}{\hbar} N(\mu) \int d\Omega \Omega \alpha^2 F_{E_{2g}}(\Omega), \tag{S6}$$

$$G_{\rm ph} = \frac{2\pi k_B}{\hbar} N(\mu) \int d\Omega \Omega \alpha^2 F_{\rm ph}(\Omega), \tag{S7}$$

and the lattice specific heats at $T = T_{\rm max}$. We have in particular $C_{E_{2g}} = 0.13 \times 10^6$ J/m$^3$K, $C_{\rm ph} = 4.1 \times 10^6$ J/m$^3$K, $G_{E_{2g}} = 2.8 \times 10^{18}$ W/m$^3$K, and $G_{\rm ph} = 3.6 \times 10^{18}$ W/m$^3$K.

With these computational inputs, we can estimate the temperature-dependent relaxation times for the electrons, and for the hot and cold phonon modes.

Given the almost linear dependence of $C_{\rm e}$ on $T_{\rm e}$, and using Eqs. (1)-(3) of the main text, we can in first approximation estimate the energy transfer rate from electron to the hot and cold lattice modes as:

$$\frac{\partial}{\partial t}\left(\frac{T_{\rm e}}{T_i}\right) = \frac{G_i}{\gamma_{\rm e} T_i}\left(1 - \frac{T_i}{T_{\rm e}}\right), \tag{S8}$$

where $i = E_{2g}$ for hot modes and $i =$ ph for cold modes.

Equation (S8) predicts an initial linear reduction in time of the electron temperature, $T_{\rm e} \approx -\alpha_i t$, towards the hot and cold lattice modes, with slopes $\alpha_{E_{2g}} = G_{E_{2g}}/\gamma_{\rm e} = 31$ K fs$^{-1}$, $\alpha_{\rm ph} = G_{\rm ph}/\gamma_{\rm e} = 40$ K fs$^{-1}$, followed by a standard (temperature-dependent) exponential decay $T_{\rm e} \approx \exp(-t/\tau_{{\rm e},i})$, where $\tau_{{\rm e},i} = \gamma_{\rm e} T_i/G_i$. With the ab initio input data reported above, we get at $T_{E_{2g}} = T_{E_{2g}}^{\rm max}$, $\tau_{{\rm e},E_{2g}} = 38$ fs, and $\tau_{\rm e,ph} = 10$ fs. The smaller value of $\tau_{\rm e,ph}$ with respect to $\tau_{{\rm e},E_{2g}}$ is consistent with the larger value of $\lambda_{\rm ph}$ compared with $\lambda_{E_{2g}}$. The crossover between the linear and exponential regime, assuming a final equilibrium temperature $T_{\rm e}^\infty = T_i^\infty \approx 400$ K is about $50 - 65$ fs, which is also visible in Fig. 2 of the main text.

More enlightening is the computation of the relaxation time of the hot and cold lattice modes towards the electronic degrees of freedom. A crucial role is played in this case by the marked difference of the corresponding lattice specific heats. More in particular, we can estimate hot and cold mode relaxation rates $\tau_i$ from the equation:

$$\frac{\partial}{\partial t}\left(\frac{T_i}{T_{\rm e}}\right) = \frac{G_i}{C_i}\left(1 - \frac{T_i}{T_{\rm e}}\right). \tag{S9}$$

Since in the relevant temperature range neither $G_i$ nor $C_i$ depend significantly on the temperature, we get the *temperature-independent* relaxation rates for the hot and cold modes: $\tau_{E_{2g}} = C_{E_{2g}}/G_{E_{2g}} = 46$ fs, $\tau_{\rm ph} = C_{\rm ph}/G_{\rm ph} = 1.1$ ps, Such large difference between $\tau_{E_{2g}}$ and $\tau_{\rm ph}$ is consistent with Fig. 2 and it reveals the establishing of hot $E_{2g}$ phonons on a picosecond scale.

In our computational framework we cannot calculate directly the relaxation time $\tau_0$ between hot and cold modes, which is ruled by anharmonic phonon-phonon terms. We take thus the value of $\tau_0 = 400$ fs from Ref. [S3] and $\delta = \lambda/4\pi k$, where $k = 3.5$ for $\lambda = 800$ nm [S4]. In addition, in the same approximation scheme as Eqs. (S1)-(S7), we can write electronic thermal conductivity as: $\kappa = \kappa_0 T_{\rm e}/(T_{\rm ph}/2 + T_{E_{2g}}/2)$, where $\kappa_0 = 26$ W/mK [S5]. The gradient term $\propto \kappa$ is actually included in our three-temperature model for the sake of completeness, and it is not expected to be relevant for thin films.

We point out that the final aim of the present analysis is to estimate the rates of the energy transfer between the different degrees of freedom. The three-temperature model represents thus just a suitable, although approximate, tool to achieve this result. One of the basic assumptions of this model is that the electrons, due to electron-electron scattering, will reach a thermal distribution with an effective temperature $T_{\rm e}$ within a shorter time-scale than the transfer to other lattice degrees of freedom, whose dynamics is dictated by the electron-phonon scattering. The effective time needed by the electrons in metals to thermalize among them is debated, ranging from tenths [S6] to hundreds of fs [S7, S8].

## S2. NON-THERMAL ELECTRON RELAXATION AND VALIDATION OF EFFECTIVE TEMPERATURE MODEL

Two- (or three-) temperature model is usually employed to describe the energy transfer dynamics between electron and lattice degrees of freedom under non-equilibrium initial condition. The implicit assumption underlying this model is that the electron-electron and the anharmonic phonon-phonon scattering leads to separate thermal distributions

with two "effective" temperatures $T_{\rm e}$, $T_{\rm L}$ on a timescale shorter than the relaxation time needed to restore the full thermal equilibrium between electron and lattice.

The actual validity of this effective-temperature model is still debated and not fully assessed. On the one hand, there is substantial evidence that in common metals electrons do not reach a thermal distributions in a shorter lapse than the relaxation time between electron and lattice degrees of freedom. On the other hand, the lack of a thermal distribution, in principle, does not necessarily affect the estimate of the relaxation times between electron and lattice degrees of freedom.

Here we introduce and employ a suitable model for studying the time-resolved dynamics of electron and lattice degrees of freedom out of equilibrium *without* assuming any thermal distribution or effective temperature. The results of this approach are compared with the results obtained from an effective two-temperature model. We show that, under the most unfavourable conditions, the lack of electron thermalization does not affect significantly the estimates of the electron-phonon relaxation time.

We consider the time evolution of generic electron and phonon populations:

$$\frac{\partial f_k}{\partial t} = -\frac{2\pi}{\hbar N}\sum_p |M_{k,p}|^2 \left\{ f_k(1-f_p)\left[(b_{k-p}+1)\delta(\epsilon_k-\epsilon_p-\hbar\omega_{k-p}) + b_{k-p}\delta(\epsilon_k-\epsilon_p+\hbar\omega_{k-p})\right] \right.$$
$$\left. - f_p(1-f_k)\left[(b_{k-p}+1)\delta(\epsilon_k-\epsilon_p+\hbar\omega_{k-p}) + b_{k-p}\delta(\epsilon_k-\epsilon_p-\hbar\omega_{k-p})\right]\right\}, \tag{S10}$$

$$\frac{\partial b_q}{\partial t} = -\frac{4\pi}{\hbar N}\sum_k |M_{k,k+q}|^2 f_k(1-f_{k+q})\left[b_q\delta(\epsilon_k-\epsilon_{k+q}+\hbar\omega_q) - (b_q+1)\delta(\epsilon_k-\epsilon_{k+q}-\hbar\omega_q)\right], \tag{S11}$$

where $f_k$, $b_q$ are the electron and phonon occupation numbers, respectively, and $M_{k,k+q}$ are the electron-phonon matrix elements (note that $q = k - p$). Eqs. (S10)-(S11) do not rely on the assumption of a thermal distribution and they are the basis of a full **k**-resolved Bloch-Boltzmann-Peierls equations employed in DFT based methods [S9].

As intermediate step between a **k**-resolved dynamics and an effective-temperature model (**k**-integrated dynamics) we consider the energy-resolved quantities:

$$f_E = \frac{1}{NN(E)}\sum_k f_k\delta(E-\epsilon_k), \tag{S12}$$

$$b_\Omega = \frac{1}{NB(\Omega)}\sum_q b_q\delta(\Omega-\omega_q), \tag{S13}$$

where $N(E)$, $B(\Omega)$ are the electron and phonon density of states, respectively.

Under the usual assumption $\alpha^2F(\epsilon,x,\Omega) \approx \alpha^2F(\Omega)$, we get thus:

$$\frac{\partial f_E}{\partial t} = -\pi\int d\Omega\alpha^2F(\Omega)\int dx f_E(1-f_x)\left[(b_\Omega+1)\delta(E-x-\hbar\Omega) + b_\Omega\delta(E-x+\hbar\Omega)\right]$$
$$+\pi\int d\Omega\alpha^2F(\Omega)\int dx(1-f_E)f_x\left[(b_\Omega+1)\delta(E-x+\hbar\Omega) + b_\Omega\delta(E-x-\hbar\Omega)\right], \tag{S14}$$

$$\frac{\partial b_\Omega}{\partial t} = -\frac{N(0)}{B(\Omega)}2\pi\alpha^2F(\Omega)\int dx\int dy$$
$$\left[f_x(1-f_y)b_\Omega\delta(x-y+\hbar\Omega) - f_x(1-f_y)(b_\Omega+1)\delta(x-y-\hbar\Omega)\right]. \tag{S15}$$

Equations (S14)-(S15) represent the starting point of our analysis. Equations (S14)-(S15), once integrated upon the electronic and phonon density of states, respectively, define the dynamics of the electron and lattice energies and, under the assumption of effective temperatures $T_{\rm e}$, $T_{\rm L}$, end up as the standard two-temperature model [S1, S2]. We proceed along an alternative path. More specifically, we use directly Eqs. (S14)-(S15) to compute the time dynamics of the electron and phonon populations *without* assuming any thermal distribution. Equations (S14)-(S15) are much more computationally affordable than Eqs. (S10)-(S11), still retaining all the useful information encoded in the energy resolution.

We employ Eqs. (S14)-(S15) on a representative example inspired by $MgB_2$. We assume a $\delta(t)$ pumping at energy 1.6 eV in a symmetric particle-hole system with constant electron density of states $N(0)$, creating particle excitations in a window $+0.8 \pm 0.005$ eV and hole excitations in a window $-0.8 \pm 0.005$ eV. The total energy pumped in the electronic degrees of freedom is thus $E_{\rm tot}(t=0) = 32 \times 10^3 N(0)$ meV$^2$, which corresponds, if fast electron thermalization would be operative, to an effective $T_{\rm e} \approx 1100$ K. We assume electron-phonon coupling with phonons in an energy window $\omega_{\rm ph} \in [60 : 70]$ meV and dimensionless coupling $\lambda = 0.26$ (which models the $E_{2g}$ hot phonon value). Consistently with the specific case of $MgB_2$, the phonon density of states $B(\Omega)$ in this range is taken to be approximatively

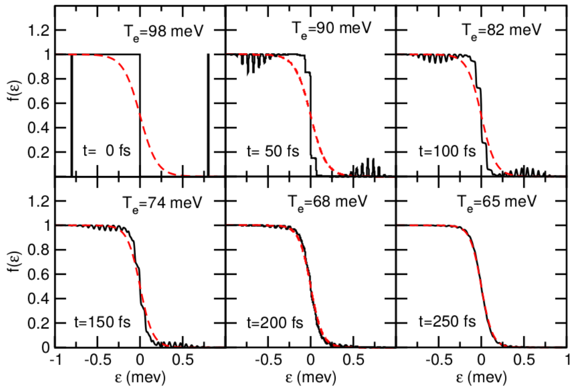


FIG. S2. Time evolution of the electronic distribution function $f_E$ for non-thermal relaxation (solid black lines). For comparison, in each panel we show also the "effective" temperature $T_e$ that would be estimated in the two-temperature model, as well as the corresponding distribution function (dashed red lines).

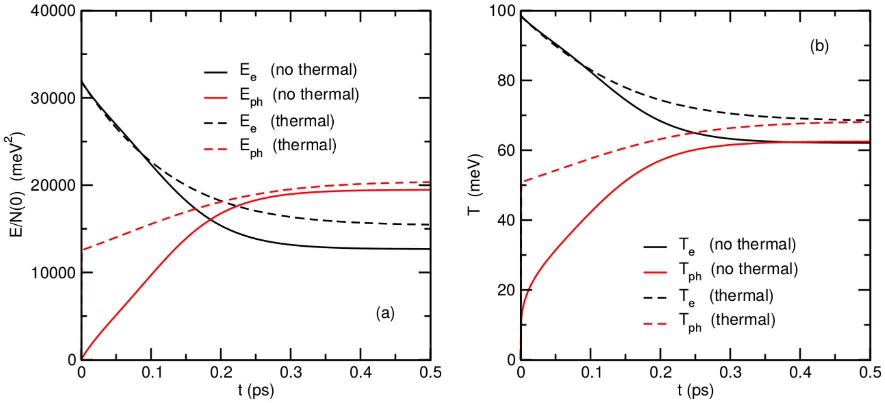


FIG. S3. Time evolution of (a) the electronic and lattice energies and of (b) the effective temperatures. In panel (b) the electronic and lattice temperatures for the model in Eqs. (S14)-(S15), in the absence of a thermal distribution, were estimated as the temperature needed in the effective two-temperature model to obtain the same electronic and lattice energies.

$B(\Omega) = 50N(0)$. Lattice modes are assumed to be at zero temperature at $t = 0$. We stress that these modelling (i.e. dispersionless particle-hole excitations, dispersionless phonon modes), due to the reduces phase space, is particularly unfavourable for final thermalization. More realistic modelling, including a dispersion of the initial particle-hole excitations, the presence of low-frequency phonons and the direct electron-electron Coulomb interaction, is expected to result in a faster dynamics towards the final equilibrium.

The plot of the time evolution of the electronic distribution is shown in Fig. S2. It is remarkable here that, although electron-electron scattering is here completely neglected, the electron-phonon interaction itself leads to an effective thermalization of the electronic degrees of freedom in a timescale of few hundredths of fs.

The timescale related to the final energy redistribution *between* electron and lattice degrees of freedom is shown in Fig. S3(a), where we compare the dynamics of electronic and lattice energies evaluated *without* the assumption of thermal distribution with the corresponding dynamics evaluated within the two-temperature model. We can see that the electronic and lattice energies reach the final asymptotic equilibrium essentially on the time scale $t \approx 0.3 - 0.4$ ps in *both* cases [S10], pointing out that the lack of a fast electronic thermal distribution due to the electron-electron interaction do not affect the estimates of the electron-phonon based relaxation times. This is evident also in Fig. S3(b), where we parametrize the electron and lattice energies evaluated from Eqs. (S14)-(S15) without the assumption of thermal distributions in terms of "effective" temperatures, i.e., the temperature that would be obtained from the same electron and lattice energies *assuming* a thermal distribution.

The lack of the idea of a fast electronic thermalization due to the Coulomb electron-electron interaction does not affect thus the estimates of the electron-phonon based relaxation times ruling the energy transfer between electronic and lattice degrees of freedom, and therefore supporting the validity of an effective temperature model.

## S3. DETAILED ANALYSIS OF STOKES AND ANTI-STOKES INTENSITIES

In Fig. 2 of the main text we displayed the time evolution of the Stokes and anti-Stokes intensity (as well their ratio) for the $E_{2g}$ mode. The strong enhancement of the anti-Stokes intensity is a direct signature of the $E_{2g}$ hot-phonon physics. This time-evolution is reproduced once more in Fig. S4a and compared in Fig. S4b with the time-dependence of the Stokes and anti-Stokes intensity intensity for the $B_{1g}$ mode, which is weakly coupled and governed thus by the cold lattice temperature $T_{\rm ph}$. We predict for the $B_{1g}$ a negligible enhancement of the Stokes intensity, and just a weak enhancement of the anti-Stokes intensity, which will be always much smaller than the Stokes intensity.

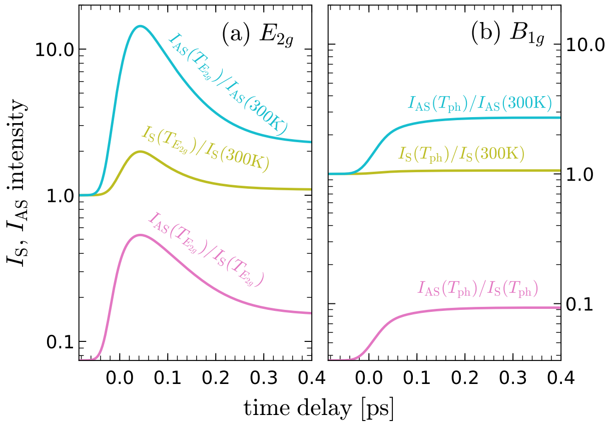


FIG. S4. Plot of the time-evolution of the anti-Stokes intensity $I_{\rm AS}(T)/I_{\rm AS}(300\,{\rm K})$, Stokes intensity $I_{\rm S}(T)/I_{\rm S}(300\,{\rm K})$, and their ratio $I_{\rm AS}(T)/I_{\rm S}(T)$, for the $E_{2g}$ hot mode (left panels) and for the $B_{1g}$ cold mode (right panel). The $E_{2g}$ mode is governed by the temperature $T = T_{E_{2g}}$ while the $B_{1g}$ mode probes the lattice temperature $T = T_{\rm ph}$.

## S4. ANALYSIS OF THE $E_{2g}$ PHONON SELF-ENERGY

In order to highlight the different physical processes that govern the time-evolution of the spectral properties of the $E_{2g}$ mode in the pump-probe setup, as depicted in Fig. 3 of the main text, we provide here a detailed analysis of the phonon self-energy and of the different mechanisms ruling it. We follow the analysis of Ref. [S11] properly generalized to the case of three different temperatures, $T_{\rm e}$, $T_{E_{2g}}$ and $T_{\rm ph}$. In this context we can write the phonon self-energy as:

$$\Pi_\nu(\omega;\{T\}) = \sum_{nm,\mathbf{k}\sigma} |g_\nu^{nm}(\mathbf{k})|^2 \int d\omega' \int d\omega'' A(\epsilon_{n\mathbf{k}},\omega';\{T\}) A(\epsilon_{m\mathbf{k}},\omega'';\{T\}) \frac{f(\omega';T_{\rm e}) - f(\omega'';T_{\rm e})}{\omega+\omega'-\omega''+i\eta}, \tag{S16}$$

where $g_\nu^{nm}(\mathbf{k})$ denotes for the mode $\nu = E_{2g}$ the electron-phonon matrix element from a state $\mathbf{k}$ on the band $n$ to a state $\mathbf{k}$ on the band $m$, $\eta$ is an infinitesimally small positive quantity, $\sigma$ is the spin index, and $A(\epsilon,\omega;\{T\})$ is the fully-interacting electronic spectral function:

$$A(\epsilon,\omega;\{T\}) = -\frac{1}{\pi}{\rm Im}\left[\frac{1}{\omega+\mu-\epsilon-\Sigma(\omega;\{T\})+i\eta}\right]. \tag{S17}$$

The electronic self-energy $\Sigma(\omega;\{T\})$ in Eq. (S17) accounts for the electron-phonon scattering with the full phonon spectrum. Its imaginary part can be written as:

$$\Sigma''(\omega;\{T\}) = -\pi \int d\Omega \alpha^2 F(\Omega)[2b(\Omega;T_\Omega) + f(\Omega-\omega;T_{\rm e}) + f(\Omega+\omega;T_{\rm e})], \tag{S18}$$

and the real part can be obtained by Kramers-Kronig transformation. Employing the model $\alpha^2F(\Omega) = \alpha^2F_{E_{2g}}(\Omega) + \alpha^2F_{\rm ph}(\Omega)$, the phonon temperature $T_\Omega$ in Eq. (S18) represents here $T_\Omega = T_{E_{2g}}$ for $\alpha^2F_{E_{2g}}(\Omega)$ and $T_\Omega = T_{\rm ph}$ for $\alpha^2F_{\rm ph}(\Omega)$.

We remind that, in order to avoid double-counting of physical processes [S12], the non-interacting adiabatic self-energy at $T = 0\,{\rm K}$ is subtracted in the definition of $\overline{\Pi}_\nu(\omega;\{T\})$ in Eq. (4) of the main text, i.e. $\overline{\Pi}_\nu(\omega;\{T\}) =$

$\Pi_\nu(\omega;\{T\}) - \Pi^0_\nu(\omega=0;\{T\}=0)$. For purpose of analysis, it is useful to split the total self-energy in an interband and intraband terms:

$$\overline{\Pi}_\nu(\omega;\{T\}) = \overline{\Pi}^{\text{inter}}_\nu(\omega;\{T\}) + \overline{\Pi}^{\text{intra}}_\nu(\omega;\{T\}). \tag{S19}$$

A further insight comes from the decomposing of each (interband/intraband) term in an adiabatic and nonadiabatic contributions [S11, S13–S15]:

$$\overline{\Pi}_\nu(\omega;\{T\}) = \overline{\Pi}^{\text{NA}}_\nu(\omega;\{T\}) + \overline{\Pi}^{\text{A}}_\nu(\{T\}), \tag{S20}$$

where $\overline{\Pi}^{\text{NA}}_\nu(\omega;\{T\}) = \Pi_\nu(\omega;\{T\}) - \Pi_\nu(\omega=0;\{T\})$, and $\overline{\Pi}^{\text{A}}_\nu(\{T\}) = \Pi_\nu(\omega=0;\{T\}) - \Pi_\nu(\omega=0;\{T\}=0)$. Notice that the adiabatic phonon self-energy is purely real and thus only contributes to the renormalization of the phonon frequency.

Note that both interband and intraband terms here result from the convolution of two fully-interacting electronic Green's functions, containing in particular the electronic damping processes determined by the imaginary part of the electronic self-energy, but also electron energy renormalization processes governed by the real part of the electronic self-energy.

The relevance of these processes is however different in the interband and in the intraband terms. The interband term involves particle-hole excitations with energies $\Delta\varepsilon_{\mathbf{k}} = |\varepsilon_{n\mathbf{k}} - \epsilon_{n\mathbf{k}}|$ ($n \neq n$ are here band indices) only above a threshold $\Delta_{\text{min}}$ dictated by the band-structure. In $MgB_2$ $\Delta_{\text{min}}$ is approximately 0.3 eV Such value is much larger than the largest electronic damping terms $\Gamma_{\text{el}} \approx 0.03$ eV [S16, S17] at $\omega \approx \Omega_{E_{2g}}$. On this ground ($\Gamma_{\text{el}} \ll \Delta_{\text{min}}$) we can safely neglect the contribution of the *imaginary* part of the electronic self-energies in the interband term. Furthermore, the *real* part of the electronic self-energies decay rapidly for energies larger than the maximum phonon frequencies. The condition $\Omega_{E_{2g}} \ll \Delta_{\text{min}}$ allows us to neglect also the real par of the electronic self-energy, implying that the interband term can be evaluate in the non-interacting case:

$$\Pi^{\text{inter}}_\nu(\omega;\{T\}) \approx \Pi^{\text{inter},0}_\nu(\omega;T_{\text{e}}) = \sum_{n\neq m,\mathbf{k}\sigma} |g^{nm}_\nu(\mathbf{k})|^2 \frac{f(\varepsilon_{n\mathbf{k}}-\mu;T_{\text{e}}) - f(\varepsilon_{m\mathbf{k}}-\mu;T_{\text{e}})}{\omega + \varepsilon_{n\mathbf{k}} - \varepsilon_{m\mathbf{k}} + i\eta}, \tag{S21}$$

Note that only $T_{\text{e}}$ appears in Eq. (S21). On the basis of Eqs. (S19)–(S21) we can further identify:

$$\overline{\Pi}^{\text{inter,NA}}_\nu(\omega;T_{\text{e}}) = -\sum_{n\neq m,\mathbf{k}\sigma} \frac{\omega\,|g^{nm}_\nu(\mathbf{k})|^2}{\varepsilon_{n\mathbf{k}} - \varepsilon_{m\mathbf{k}}} \frac{f(\varepsilon_{n\mathbf{k}}-\mu;T_{\text{e}}) - f(\varepsilon_{m\mathbf{k}}-\mu;T_{\text{e}})}{\omega + \varepsilon_{n\mathbf{k}} - \varepsilon_{n\mathbf{k}} + i\eta}, \tag{S22}$$

$$\overline{\Pi}^{\text{inter,A}}_\nu(T_{\text{e}}) = \sum_{n\neq m,\mathbf{k}\sigma} |g^{nm}_\nu(\mathbf{k})|^2 \left[\frac{f(\varepsilon_{n\mathbf{k}}-\mu;T_{\text{e}}) - f(\varepsilon_{m\mathbf{k}}-\mu;T_{\text{e}})}{\varepsilon_{n\mathbf{k}} - \varepsilon_{m\mathbf{k}} + i\eta} - \frac{f(\varepsilon_{n\mathbf{k}}-\mu;0) - f(\varepsilon_{m\mathbf{k}}-\mu;0)}{\varepsilon_{n\mathbf{k}} - \varepsilon_{m\mathbf{k}} + i\eta}\right]. \tag{S23}$$

Since we are interested in $\omega \approx \Omega_{E_{2g}}$, and, as said, the excitations $\varepsilon_{n\mathbf{k}} - \varepsilon_{m\mathbf{k}}$ have a minimum threshold $\Delta_{\text{min}}$, it is clear that the nonadiabatic term can be neglected in the regime $\Omega_{E_{2g}} \ll \Delta_{\text{min}}$, which is representative of $MgB_2$. On the other hand, the adiabatic interband term is usually negligible at room temperature ($T \ll \Delta_{\text{min}}$) under conventional steady conditions, but it becomes highly relevant in pump-probe experiments where the transient electronic temperature $T_{\text{e}}$ can be as large as the optical threshold $\Delta_{\text{min}}$.

Just as in the interband term, a similar level of approximation (i.e. neglecting the electronic self-energy in the electronic Green's functions) is often enforced [S13, S14] also in the computation of the intraband term in Eq. (S20), and the approximate expression is employed:

$$\Pi^{\text{intra}}_\nu(\omega;\{T\}) \approx \Pi^{\text{intra},0}_\nu(\omega;\{T\}) = -\sum_{n\mathbf{k}\sigma} |g^{nn}_\nu(\mathbf{k})|^2 \left[\frac{\partial f(\varepsilon_{n\mathbf{k}}-\mu;T_{\text{e}})}{\partial\varepsilon_{n\mathbf{k}}}\right]. \tag{S24}$$

This approximation is rather robust in graphene and in the physical cases discussed in Refs. [S13, S14], but it is known to miss relevant physics in $MgB_2$ where the electronic damping processes can govern the phonon damping [S11, S18]. In this context, the fully-interacting spectral representation for the electronic Green's functions as shown in Eq. (S16) must be employed.

From a computational point of view, following similar approaches developed for the optical conductivity [S19–S23], Eq. (S16) can be very well approximated with great accuracy by the compact expression [S11]:

$$\Pi^{\text{intra}}_\nu(\omega;\{T\}) = \sum_{n\mathbf{k}\sigma} |g^{nn}_\nu(\mathbf{k})|^2 \left[\frac{\partial f(\epsilon_{n\mathbf{k}}-\mu;T_{\text{e}})}{\partial\epsilon_{n\mathbf{k}}}\right] \frac{\omega\lambda(\omega;\{T\}) + i\gamma(\omega;\{T\})}{\omega[1+\lambda(\omega;\{T\})] + i\gamma(\omega;\{T\})}, \tag{S25}$$

where [S11, S20, S21]

$$\gamma(\omega;\{T\}) = \frac{\pi}{\omega}\int d\Omega\alpha^2F(\Omega)\int d\varepsilon\,[f(\varepsilon;T_\mathrm{e}) - f(\varepsilon+\omega;T_\mathrm{e})]$$
$$\times\,[4b(\Omega;T_\Omega) + f(\Omega+\varepsilon+\omega;T_\mathrm{e}) + f(\Omega-\varepsilon-\omega;T_\mathrm{e}) + f(\Omega+\varepsilon;T_\mathrm{e}) + f(\Omega-\varepsilon;T_\mathrm{e})] \tag{S26}$$
$$= \frac{\pi}{\omega}\int d\Omega\alpha^2F(\Omega)\left[2\omega\coth\frac{\Omega}{2k_BT_\Omega} - (\omega+\Omega)\coth\frac{\omega+\Omega}{2k_BT_\mathrm{e}} + (\omega-\Omega)\coth\frac{\omega-\Omega}{2k_BT_\mathrm{e}}\right]. \tag{S27}$$

Note that the appearing of an electronic or lattice temperature in Eq. (S27) is unambiguously dictated by the Fermi o Bose thermal factor. The quantity $\omega\lambda(\omega;\{T\})$ can be obtained here upon Kramers-Kronig transformation of $\gamma(\omega;\{T\})$.

Eq. (S27) is crucially helpful in our analysis. Writing $\alpha^2F(\Omega) = \alpha^2F_{E_{2g}}(\Omega) + \alpha^2F_\mathrm{ph}(\Omega)$, we can express the optical damping function $\gamma(\omega;\{T\})$ as a sum of three independent contributions depending separately on each temperature $T_\mathrm{e}$, $T_{E_{2g}}$, $T_\mathrm{ph}$:

$$\gamma(\omega;\{T\}) = \gamma_\mathrm{e}(\omega;T_\mathrm{e}) + \gamma_{E_{2g}}(T_{E_{2g}}) + \gamma_\mathrm{ph}(T_\mathrm{ph}), \tag{S28}$$

where

$$\gamma_\mathrm{e}(\omega;T_\mathrm{e}) = -\frac{\pi}{\omega}\int d\Omega\alpha^2F(\Omega)\left[(\omega+\Omega)\coth\frac{\omega+\Omega}{2k_BT_\mathrm{e}} - (\omega-\Omega)\coth\frac{\omega-\Omega}{2k_BT_\mathrm{e}}\right], \tag{S29}$$

$$\gamma_{E_{2g}}(T_{E_{2g}}) = 2\pi\int d\Omega\alpha^2F_{E_{2g}}(\Omega)\coth\frac{\Omega}{2k_BT_{E_{2g}}}, \tag{S30}$$

$$\gamma_\mathrm{ph}(T_\mathrm{ph}) = 2\pi\int d\Omega\alpha^2F_\mathrm{ph}(\Omega)\coth\frac{\Omega}{2k_BT_\mathrm{ph}}. \tag{S31}$$

Note that, from this analysis, employing Kramers-Kronig transformations, the function $\lambda(\omega;\{T\})$ results to depend only on the quantity $\gamma_\mathrm{e}(\omega;T_\mathrm{e})$, and thus only on the electronic temperature: $\lambda(\omega;\{T\}) = \lambda_\mathrm{e}(\omega;T_\mathrm{e})$.

A similar decomposition can be employed also for intraband part of the optical conductivity.

In our context we use Eqs. (S19), (S20), and (S25) to get the final expressions for the nonadiabatic and adiabatic intraband phonon self-energies:

$$\overline{\Pi}_\nu^{\mathrm{intra,NA}}(\omega;\{T\}) = -\sum_{n\mathbf{k}\sigma}|g_\nu^{nn}(\mathbf{k})|^2\left[\frac{\partial f(\epsilon_{n\mathbf{k}}-\mu;T_\mathrm{e})}{\partial\epsilon_{n\mathbf{k}}}\right]\frac{\omega}{\omega[1+\lambda(\omega;\{T\})]+i\gamma(\omega;\{T\})}, \tag{S32}$$

$$\overline{\Pi}_\nu^{\mathrm{intra,A}}(T_\mathrm{e}) = \sum_{n\mathbf{k}\sigma}|g_\nu^{nn}(\mathbf{k})|^2\left[\frac{\partial f(\varepsilon_{n\mathbf{k}}-\mu;T_\mathrm{e})}{\partial\varepsilon_{n\mathbf{k}}}\right] - \sum_{n\mathbf{k}\sigma}|g_\nu^{nn}(\mathbf{k})|^2\left[\frac{\partial f(\varepsilon_{n\mathbf{k}}-\mu;0)}{\partial\varepsilon_{n\mathbf{k}}}\right]. \tag{S33}$$

Finally, the phonon self-energy $\overline{\Pi}_\nu(\omega;\{T\})$ used in the main text is composed from Eqs. (S22), (S23), (S32), and (S33).

## S5. ENERGY RESOLUTION IN THE LIGHT OF TIME-ENERGY UNCERTAINTY

In Fig. 3 of the main paper, we discuss the time evolution of the optical features of the $E_{2g}$ resonance. A frequency shift and a linewidth narrowing of $\sim 15$ meV are there predicted. The actual possibility of observing such dynamics need to face the limitations dictated by the time-energy uncertainty principle, i.e., $\Delta t\cdot\Delta E \approx 14.7\,\mathrm{cm}^{-1}\mathrm{ps}$ [S24].

Here we discuss briefly how the limitations due to the time-energy uncertainty do not prevent the possibility of detecting the predicted behavior.

If we consider $\Delta t \sim 50$ fs as the needed time resolution to trace the dynamics of the optical features, we can estimate $\Delta E \sim 36$ meV as energy resolution [S24]. Such loss of energy resolution can be modelled by convoluting our theoretical spectra with a corresponding Gaussian with the full-width-at-half-maximum (FWHM) of $\Delta E$ (in the same way we convolute the time with 50 fs Gaussian). This would actually prevent the possibility of detecting fine energy structures with energy $< \Delta E$. In case of isolated resonances, things are however much easier. The loss of energy resolution would not prevent to trace down the shift of the center of phonon peak, neither to detect sizable narrowing of the intrinsic linewidth on top of a constant line broadening due to the energy uncertainty.

The suitability of this scenario was proven for instance in Ref. [S25] in the analysis of the phonon modes in Sb single crystals.

We investigate the effects of the time-energy uncertainty by convoluting the spectra in Fig. 3 with Gaussians having FWHM of $\Delta E = 36\,\mathrm{meV}$ and $\Delta t = 50\,\mathrm{fs}$. The results are shown in Fig. S5. We can see that the loss of the energy resolution would affect only weakly the determination of the center peak, whereas it results in just an additional constant broadening in the linewidth. The time evolution of the two quantities can be still identified in a reliable way.

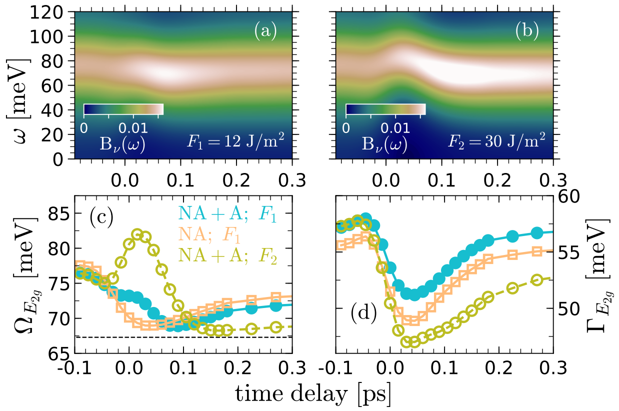


FIG. S5. Time evolution of the spectral phonon intensity and of the main optical features as in Fig. 3 of the main text, after convolution with proper Gaussians simulating the energy-time uncertainty.

* dino.novko@gmail.com
† emmanuele.cappelluti@ism.cnr.it

[S1] P. B. Allen, Phys. Rev. Lett. **59**, 1460 (1987).
[S2] Z. Lin, L. V. Zhigilei, and V. Celli, Phys. Rev. B **77**, 075133 (2008).
[S3] A. Shukla, M. Calandra, M. d'Astuto, M. Lazzeri, F. Mauri, C. Bellin, M. Krisch, J. Karpinski, S. M. Kazakov, J. Jun, D. Daghero, and K. Parlinski, Phys. Rev. Lett. **90**, 095506 (2003).
[S4] A. Balassis, E. V. Chulkov, P. M. Echenique, and V. M. Silkin, Phys. Rev. B **78**, 224502 (2008).
[S5] E. Bauer, C. Paul, S. Berger, S. Majumdar, H. Michor, M. Giovannini, A. Saccone, and A. Bianconi, Journal of Physics: Condensed Matter **13**, L487 (2001).
[S6] S. Brorson, A. Kazeroonian, S. Moodera, D. Face, T. Cheng, E. Ippen, M. Dresselhaus, and G. Dresselhaus, Phys. Rev. Lett. **64**, 2172 (1990).
[S7] W. Fann, R. Storz, H. Tom, and J. Bokor, Phys. Rev. B **46**, 13592 (1992).
[S8] J. Hohlfeld, S.-S. Wellershoff, J. Güdde, U. Conrad, V. Jähnke, and E. Matthias, Chem. Phys. **251**, 237 (2000).
[S9] S. Butscher, F. Mildea, M. Hirtschulz, E. Malić, and A. Knorr, Appl. Phys. Lett. **91**, 203103 (2007).
[S10] The final asymptotic electron/lattice energy and temperature in the two-temperature model differs from the numerical solution of Eqs. (S14)-(S15) because of having neglected the temperaure dependence of the lattice specific heat. Note however that, although this approximation leads to different final energies and temperatures, it does not affect the characteristic time scales.
[S11] D. Novko, Phys. Rev. B **98**, 041112 (2018).
[S12] F. Giustino, Rev. Mod. Phys. **89**, 015003 (2017).
[S13] M. Lazzeri and F. Mauri, Phys. Rev. Lett. **97**, 266407 (2006).
[S14] A. M. Saitta, M. Lazzeri, M. Calandra, and F. Mauri, Phys. Rev. Lett. **100**, 226401 (2008).
[S15] F. Caruso, M. Hoesch, P. Achatz, J. Serrano, M. Krisch, E. Bustarret, and F. Giustino, Phys. Rev. Lett. **119**, 017001 (2017).
[S16] V. Guritanu, A. Kuzmenko, D. van der Marel, S. Kazakov, N. Zhigadlo, and J. Karpinski, Phys. Rev. B **73**, 104509 (2006).
[S17] D. Di Castro, M. Ortolani, E. Cappelluti, U. Schade, N. Zhigadlo, and J. Karpinski, Phys. Rev. B **73**, 174509 (2006).
[S18] E. Cappelluti, Phys. Rev. B **73**, 140505 (2006).
[S19] P. B. Allen, Phys. Rev. B **3**, 305 (1971).
[S20] P. B. Allen and R. Silberglitt, Phys. Rev. B **9**, 4733 (1974).
[S21] S. Shulga, O. Dolgov, and E. Maksimov, Physica C **178**, 266 (1991).
[S22] M. Norman and A. Chubukov, Phys. Rev. B **73**, 140501 (2006).
[S23] D. Novko, Nano Lett. **17**, 6991 (2017).
[S24] R. Versteeg, J. Zhu, P. Padmanabhan, C. Boguschewski, R. German, M. Goedecke, P. Becker, and P. M. van Loosdrecht, Struct. Dyn. **5**, 044301 (2018).

[S25] D. Fausti, O. Misochko, and P. van Loosdrecht, Phys. Rev. B **80**, 161207 (2009).
